# Supplementary material for: FacePlex: Toward Natural Full-Duplex Conversational Avatars
Source: arXiv:2606.30145 source file (2026-09-28)
Supplement: Supplementary file 3 [file 1.tex]

# Paper text — future-context analysis (Figure: hidden-time correlation / window extension / trained controls)

## Figure caption (main text)

**Figure X. Speaking motion depends on the next 80–240 ms of the speech model's hidden state; listening motion does not.**
All panels share the same time axis: the offset of a hidden state h_{T+k} relative to the motion frame T (k·80 ms; positive = future).
The shaded band marks the conditioning window used by our model, [h_T, …, h_{T+3}].
**(a)** Held-out R² of a ridge probe that predicts the ground-truth motion at frame T from a *single* hidden state h_{T+k}, on Seamless Interaction (1,100 clips, 16 s each; see Supp. §S1). Speaking-frame jaw (and expression) is explained best by h_{T+1}…h_{T+3}; listening-frame head pose is not explained by any offset.
**(b)** The same probe with a *window* of hidden states, extended from h_T either into the future ([h_T … h_{T+x}]) or into the past ([h_{T−x} … h_T]). Future slots add explained variance (0.22 → 0.40 with one slot, saturating at three = our window); past slots add none.
**(c)** Lip-sync of flow-matching motion models trained with the same recipe but with the 4-slot window shifted from the past to the future (S-LVE, lower is better; PLRS, higher is better; seamless, n = 500). The dotted line is our model evaluated with its future slots left empty at inference. Quality follows the data-side curves and saturates at a lookahead of 240 ms.
Because the speech model emits h_{T+1} only after reading the audio codes of frame T (acoustic codebooks are delayed by one more step), a window ending at h_T contains no information about the sound being produced at T.

## Supplementary §S1 — Data-side analysis of future dependence

**Data.** We use the validation split of Seamless Interaction that was never used to train the motion model: 550 dyadic sessions, both participants, i.e. 1,100 clips of 16 s. For every clip we have (i) ground-truth FLAME motion at 25 fps (108-D: 100 expression, 3 head rotation, 1 jaw, 4 gaze), (ii) the participant's own and the partner's 16 kHz audio, and (iii) the hidden states of the full-duplex speech LM (PersonaPlex-7B, Moshi architecture) obtained by teacher-forcing the real conversation through the model: the participant's speech on the model's own stream and the partner's speech on the user stream. Hidden states are the 4096-D temporal-transformer outputs at 12.5 Hz (one per 80 ms frame), exactly the conditioning our motion model receives at inference. Motion is averaged over the two 25-fps frames of each 80 ms step so that motion and hidden states share one clock.

**Timing convention.** The transformer at step s reads the token row at position s − 1, and the acoustic codebooks are delayed by one frame relative to the semantic codebook. Hence h_T has read the participant's semantic codes up to frame T − 1 and acoustic codes up to T − 2; h_{T+1} is the first state that contains the sound of frame T, and h_{T+2} the first that contains its acoustic detail. All offsets are reported in hidden-state time; in audio time the peak of (a) lies 80–160 ms earlier.

**Frame classes.** A frame is *speaking* if the participant's own audio RMS exceeds 0.003 (the threshold used by the benchmark), and *listening* if the participant is silent and the partner's RMS exceeds 0.003. Frames satisfying neither are excluded.

**Probe.** For each offset k ∈ {−6, …, +6} we fit a ridge regression from h_{T+k} (standardized per dimension) to the motion at frame T. Targets are standardized per clip (each clip's mean and standard deviation removed) so that the probe measures timing information rather than a participant's average pose. Clips are split 70 / 10 / 20 % into train / validation / test; the ridge coefficient is fit on the train clips, the regularization strength is chosen on the validation clips from {10¹, …, 10⁵}, and we report R² = 1 − SSE/SST on the **held-out** test clips. R² is computed jointly over the dimensions of a target group (jaw; expression 0–99; head 100–102; gaze 103–106). For panel (b) the hidden state of each slot is first reduced to 512 dimensions by PCA fitted on training clips, and the slots of a window are concatenated before ridge regression; alpha selection and held-out evaluation are as above. Held-out R² is a lower bound on the information the hidden states carry, since the probe is linear and sees no context beyond the window.

**Trained controls (panel c).** Nine motion models were trained with one recipe (initialized from the adopted asymmetric-schedule checkpoint, 100k steps, learning rate 5·10⁻⁵, single-chunk windows, evaluated with K = 4 refinement passes) that differ only in the position of their 4-slot conditioning window: [h_{T−3−j} … h_{T−j}] for j = 6, 3, 2, 1 (windows entirely in the past), the causal window [h_{T−3} … h_T], and [h_{T−2} … h_{T+1}], [h_{T−1} … h_{T+2}], [h_T … h_{T+3}] (ours); two further models extend the window to five and six slots ([h_T … h_{T+4}], [h_T … h_{T+5}]). All are evaluated on the same 500 seamless windows (seed 20260426, full audio rollout capped at 288 motion frames, paired). Training-seed noise for this recipe is ≈ 0.35 mm S-LVE and ≈ 0.002 PLRS (three seeds of the [h_T … h_{T+3}] model: 7.09 / 6.74 / 6.94 mm), so S-LVE differences among windows reaching ≥ 160 ms are within noise and only PLRS separates them. The dotted reference (S-LVE 9.40, PLRS 0.171) is the adopted model with its three future slots left empty at inference.

**Additional observations (not in the figure).** With raw 40-band log-mel of the participant's own audio as the input instead of hidden states, the speaking-jaw probe peaks sharply at 0–80 ms (r = 0.37) and falls below r = 0.13 outside ±160 ms, confirming the 80–160 ms shift between audio time and hidden-state time. Listening-frame jaw shows a weak, broad dependence (r ≈ 0.2, slightly higher for future states) that we attribute to silent mouth preparation before the next turn; listening head pose and gaze show none (R² ≤ 0) for single states, for 1-s windows of partner speech, and for windows extended in either direction. Data files: `outputs/analysis/paper_csv/fig_{a,b,c}_*.csv`, `window_ablation_all.csv`; scripts: `scripts/analysis/{audio_time_correlation*.py, future_context_hidden_time.py, audio_window_dose_response.py}`.
