# Supplementary material for: FacePlex: Toward Natural Full-Duplex Conversational Avatars
Source: arXiv:2606.30145 source file (2026-09-28)
Supplement: Supplementary file 4 [file ablation_latency_supplement.tex]

% Run-ahead output-availability comparison, moved from the main paper.
\begin{table}[H]
    \centering
    \fontsize{8}{9}\selectfont
    \caption{Mean server-side audio/motion availability delay. Measurements include input capture and queue accumulation and exclude rendering, network transfer, and client presentation. The main-table input-plus-forward latency is 0.122\,s.}
    \label{tab:ablation_run_ahead_latency}
    \setlength{\tabcolsep}{3pt}
    \renewcommand{\arraystretch}{1.05}
    \input{Tables/tab_ablation_run_ahead_latency}
\end{table}
